# Supplementary material for: Scaling Whole-Body Human Musculoskeletal Behavior Emulation for Specificity and Diversity
Source: arXiv:2603.29332 source file (2026-03-31)
Supplement: Supplementary file 1 [file appendix.tex]

\newcommand{\extendeddatasection}[1]{%
  \section{Extended Data}%
  \setcounter{figure}{0}%
  \setcounter{table}{0}%
  \renewcommand{\thefigure}{\arabic{figure}}%
  \renewcommand{\thetable}{\arabic{table}}%
  \renewcommand{\figurename}{Extended Data Fig.}%
  \renewcommand{\tablename}{Extended Data Table}%
}

\newpage
\extendeddatasection{}

\begin{figure}[h]
    \centering
    \caption{\textbf{xxx} .}
    \label{ext_figxxx}
\end{figure}

\begin{table}[h]

\begin{tabular}{| l | l | c | c |}
\hline

\hline
\end{tabular}
\caption{xxx.}
\label{ext_tablexxx}
\end{table}
